# Supplementary material for: Artificial Microsaccade Compensation: Stable Vision for an Ornithopter
Source: arXiv:2512.03995 source file (2025-12-03)
Supplement: Supplementary file 1 [file supplemental.tex]

\section*{Supplementary Material}
\setcounter{equation}{0}

\subsection*{Supplementary Movie 1}
Supplementary Movie 1 compares stabilization results on sequence UD.

\subsection*{Supplementary Movie 2}
Supplementary Movie 2 compares stabilization results on sequence LR.

\subsection*{Supplementary Movie 3}
Supplementary Movie 3 compares stabilization results on sequence FB.

\subsection*{Supplementary Movie 4}
Supplementary Movie 4 compares stabilization results on sequence Yaw.

\subsection*{Supplementary Movie 5}
Supplementary Movie 5 compares stabilization results on sequence Circle1.

\subsection*{Supplementary Movie 6}
Supplementary Movie 6 compares stabilization results on sequence Circle2.

\subsection*{Supplementary Movie 7}
Supplementary Movie 7 compares stabilization results on sequence FF1.

\subsection*{Supplementary Movie 8}
Supplementary Movie 8 compares stabilization results on sequence FF2.

\subsection*{Supplementary Movie 9}
Supplementary Movie 9 compares stabilization results on sequence FF3.

\subsection*{Supplementary Movie 10}
Supplementary Movie 10 compares stabilization results on sequence Hand.

\subsection*{Supplementary Movie 11}
Supplementary Movie 11 compares stabilization results on sequence Hall.

\subsection*{Supplementary Movie 12}
Supplementary Movie 12 compares stabilization results on sequence Stairs.

\subsection*{Supplementary Movie 13}
Supplementary Movie 13 compares stabilization results on sequence Atrium1.

\subsection*{Supplementary Movie 14}
Supplementary Movie 14 compares stabilization results on sequence Atrium2

\subsection*{Supplementary Movie 15}
Supplementary Movie 15 compares stabilization results on sequence Lab.
